# Supplementary material for: LHCb PDF measurements
Source: arXiv:1601.00337 source file (2016-01-03)
Supplement: Supplementary file 1 [file supplementary.pdf]

# 1 Supplementary material for LHCb-PAPER-2015-001

This appendix contains supplementary material that will posted on the public cds record but will not appear in the paper.

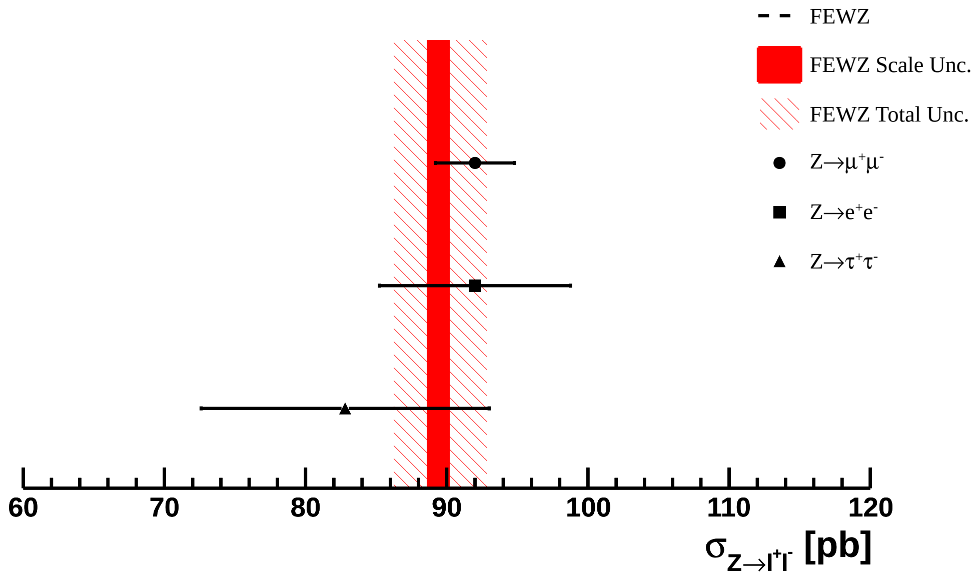


Figure 1: Comparison of LHCb $Z$ cross-section measurements to theoretical prediction. The uncertainty due to the beam energy is not displayed.

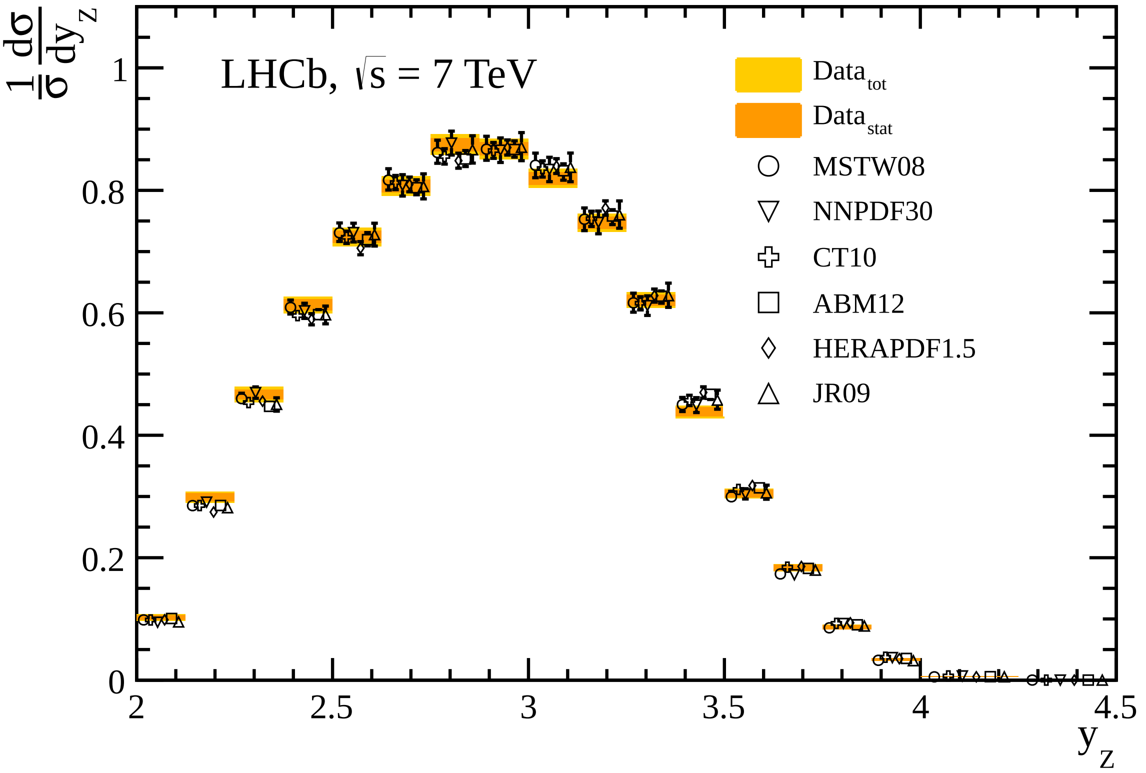


Figure 2: Normalised differential cross-section as a function of $y_Z$. The shaded (yellow) bands indicate the measurements. These are compared to FEWZ with various PDF sets.

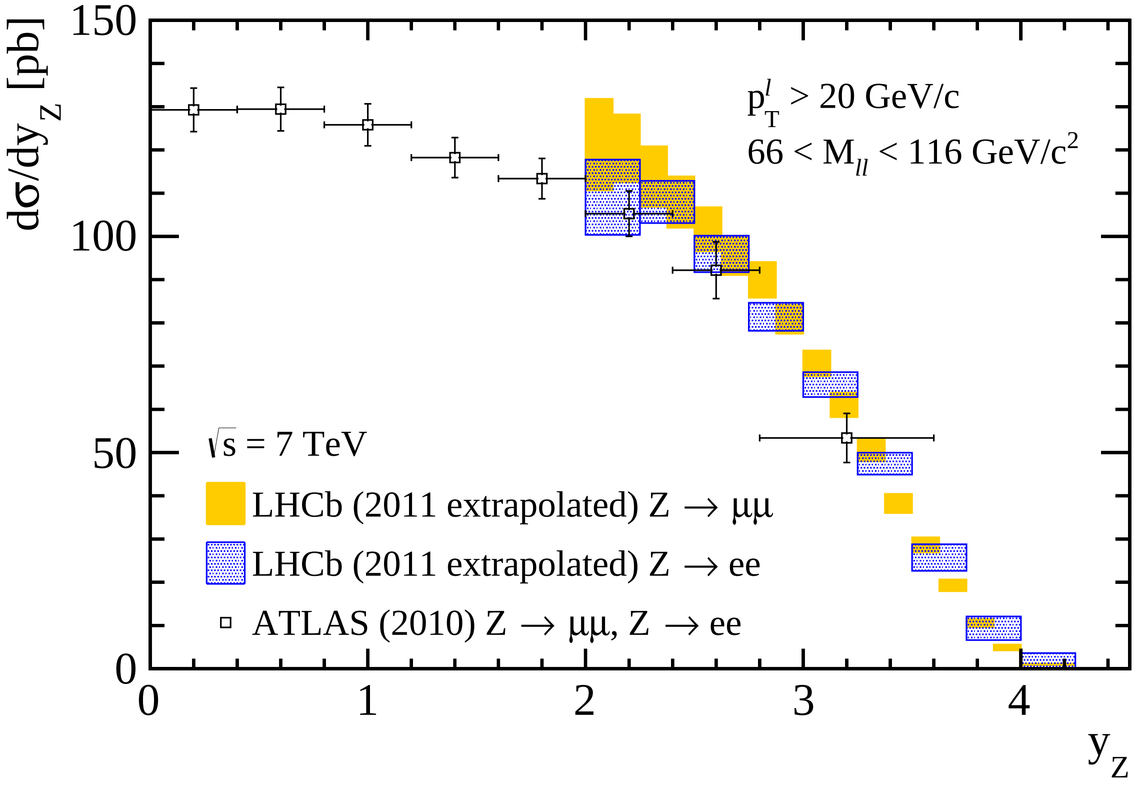


Figure 3: Extrapolation of LHCb $Z$ boson cross-section measurements to the ATLAS fiducial volume (muons with $p_{\mathrm{T}} > 20$ GeV/$c$ and invariant mass $66 < M_{\mu\mu} < 116$ GeV/$c^2$) [1].

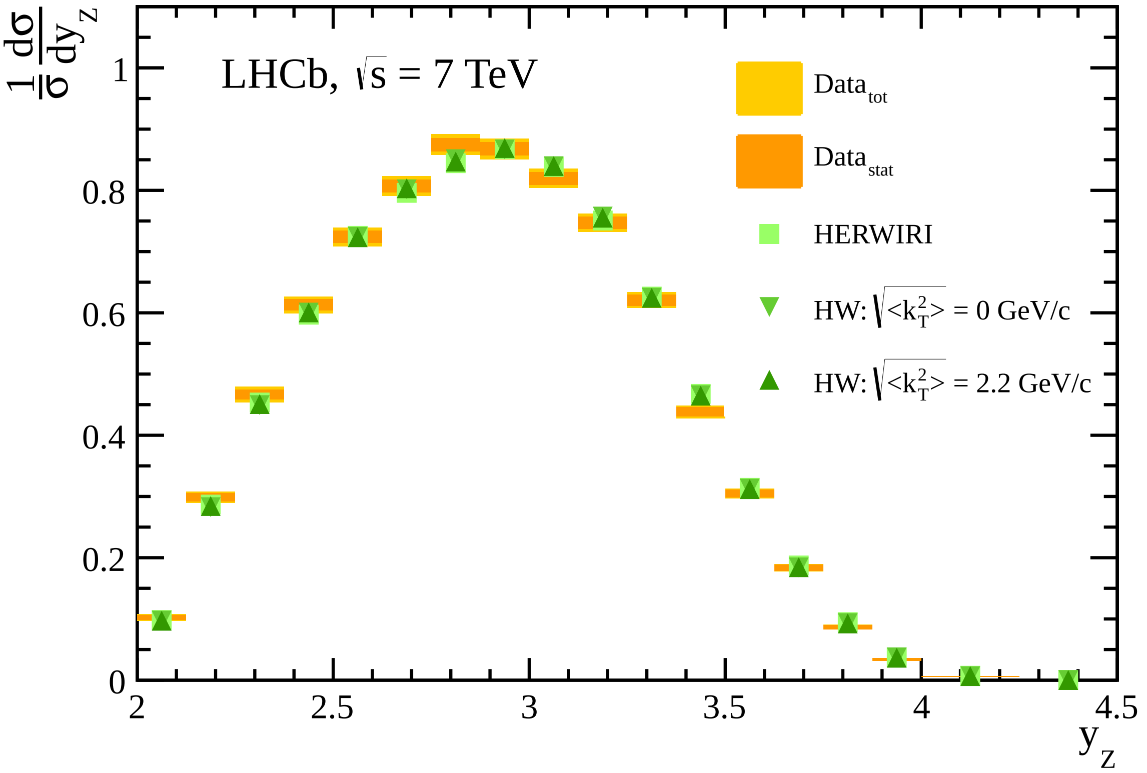


Figure 4: Normalised differential cross-section as a function of $Z$ boson $y$. The shaded (yellow) bands indicate the measurements, which are compared to MC@NLO + Herwiri (HERWIRI) and MC@NLO + Herwig (HW). Herwig is configured with two choices of the root mean-square-deviation of the intrinsic $k_T$ distribution, 0 and 2.2 GeV/$c$.

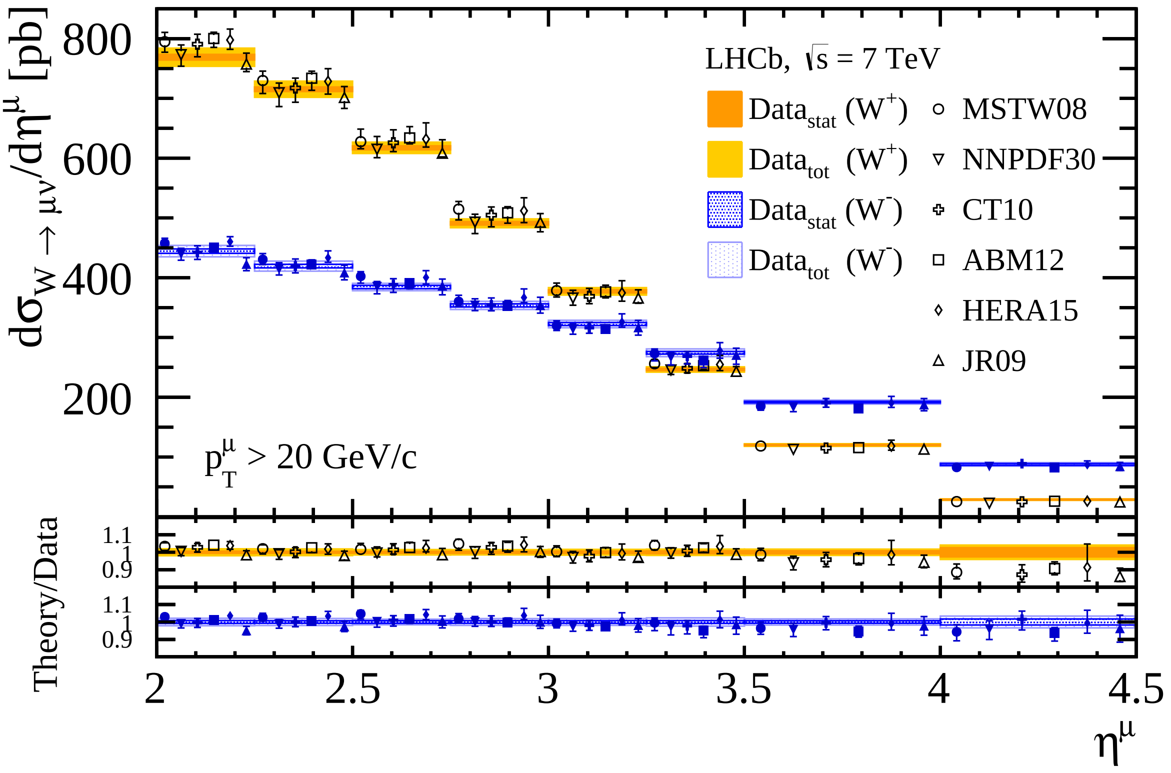


Figure 5: Differential $W^+$ and $W^-$ cross-sections as a function of muon $\eta$. Measurements, represented as bands corresponding to the statistical (orange (blue) for $W^+$ ($W^-$)) and total (yellow (light blue) for $W^+$ ($W^-$)) uncertainty, are compared to NNLO predictions with different parameterisations of the PDFs (black (blue) markers for $W^+$ ($W^-$)), displaced horizontally for presentation.

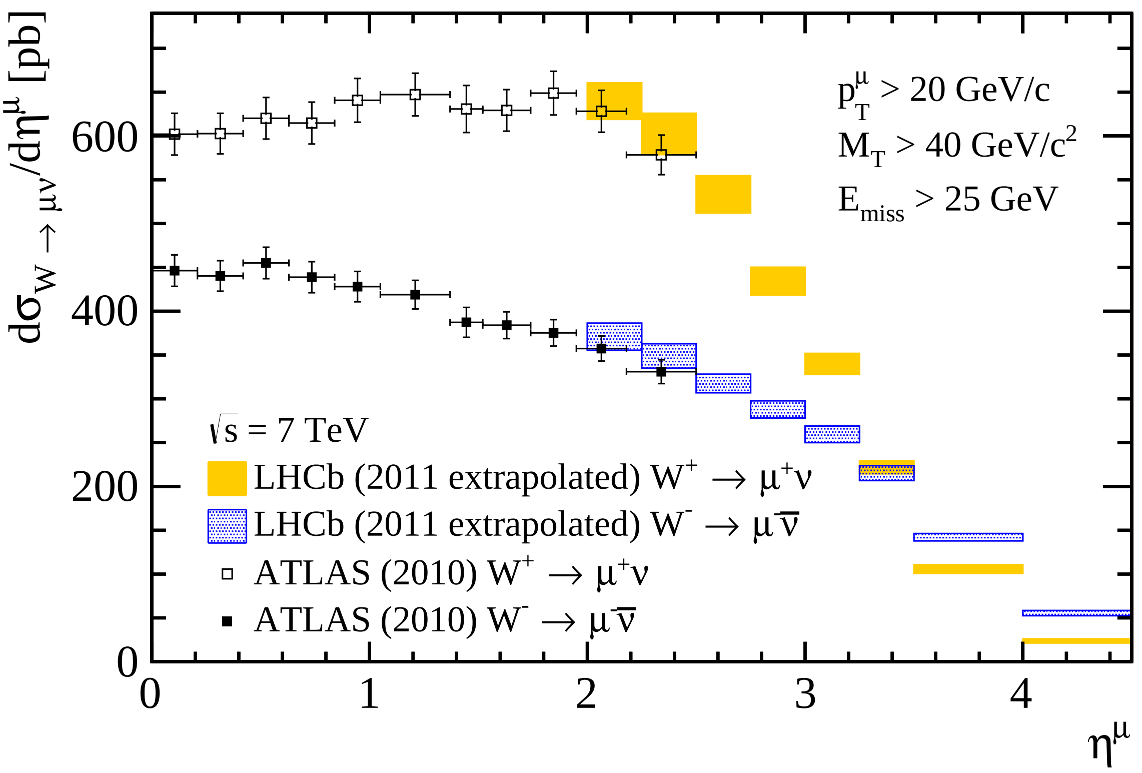


Figure 6: Extrapolation of LHCb $W$ boson cross-section measurements to the ATLAS fiducial volume (muons with $p_{\mathrm{T}} > 20$ GeV/$c$ and invariant mass $66 < M_{\mu\mu} < 116$ GeV/$c^2$) [1].

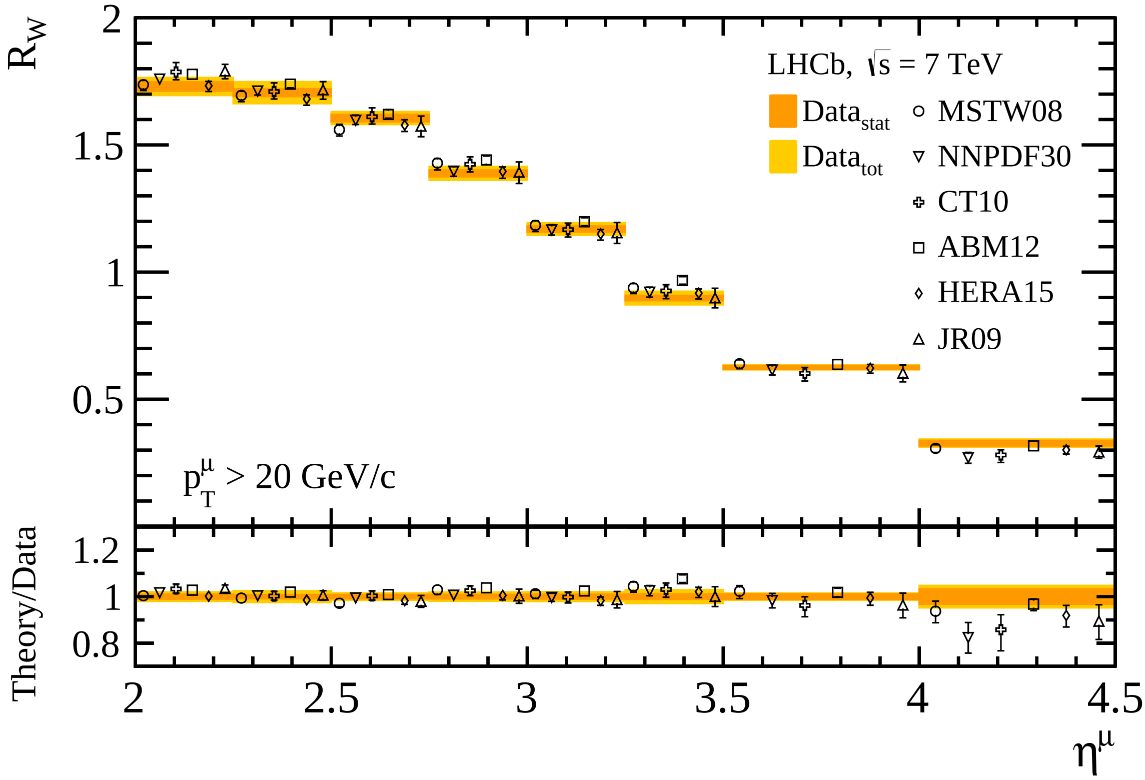


Figure 7: $W^+$ to $W^-$ cross-section ratios as a function of muon $\eta$. Measurements, represented as bands corresponding to the (orange) statistical and (yellow) total uncertainty, are compared to (black markers, displaced horizontally for presentation) NNLO predictions with different parameterisations of the PDFs.

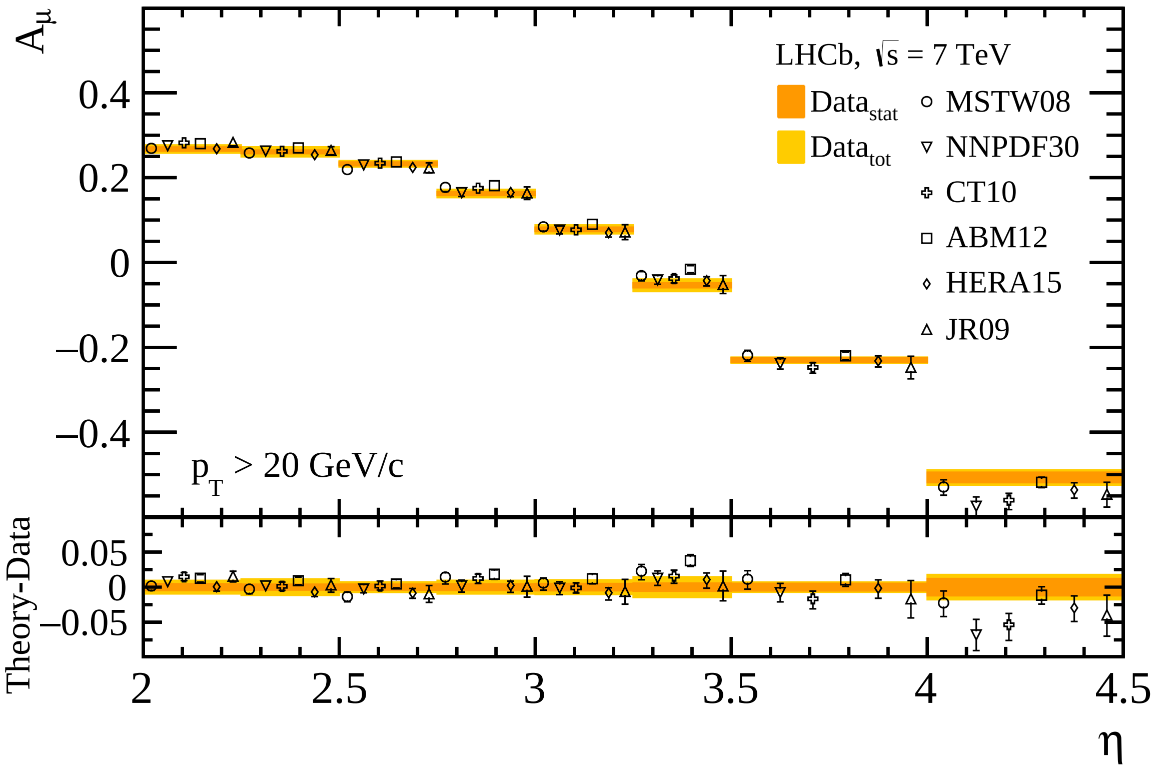


Figure 8: Lepton charge asymmetries in $W$ decays as a function of muon $\eta$. Measurements, represented as bands corresponding to the (orange) statistical and (yellow) total uncertainty, are compared to (open black markers, displaced horizontally for presentation) NNLO predictions with different parameterisations of the PDFs.

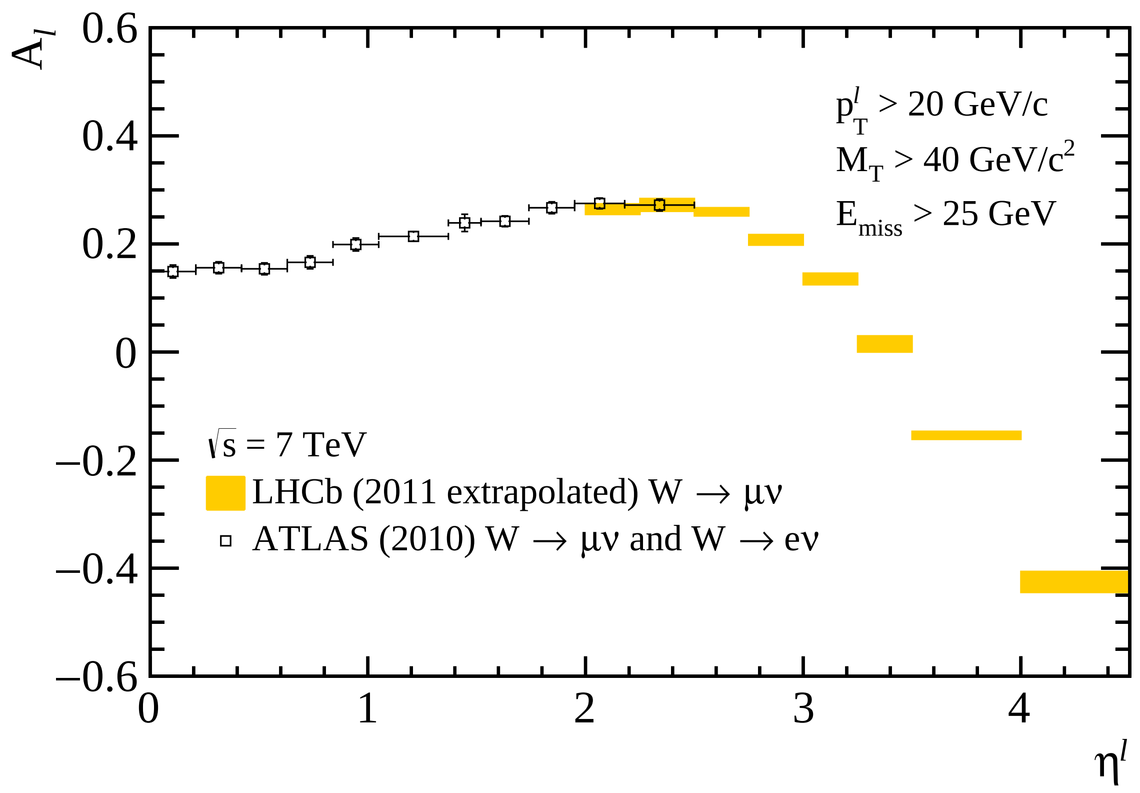


Figure 9: Lepton charge asymmetries in $W$ decays as a function of muon $\eta$. Measurements, represented as bands corresponding to the (yellow) total uncertainty, are extrapolated to the ATLAS fiducial volume ($M_{\mathrm{T}} > 40\,\mathrm{GeV}/c^2$ and $E_{\mathrm{miss}} > 25\,\mathrm{GeV}$) and compared to the (open black markers) ATLAS determinations [1].

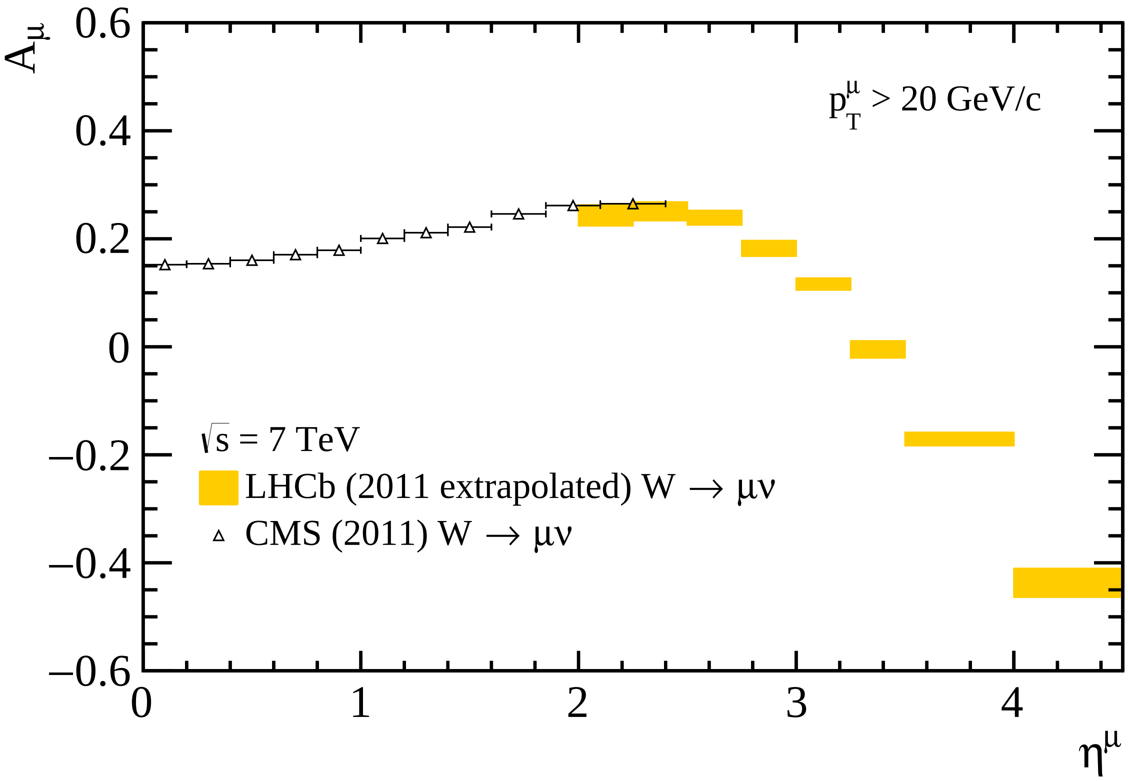


Figure 10: Lepton charge asymmetries in $W$ decays as a function of muon $\eta$. Measurements, represented as bands corresponding to the (yellow) total uncertainty, are extrapolated to the CMS fiducial volume ($p_{\mathrm{T}} > 25\,\mathrm{GeV}/c$) and compared to the (open black markers) CMS determinations [2].

# References


[1] ATLAS collaboration, G. Aad *et al.*, *Measurement of the inclusive $W^{\pm}$ and $Z/\gamma^{*}$ cross sections in the e and $\mu$ decay channels in pp collisions $\sqrt{s}$ = 7 TeV with the ATLAS detector*, Phys. Rev. D **85** (2012) 072004, `arXiv:1109.5141`.

[2] CMS collaboration, S. Chatrchyan *et al.*, *Measurement of the muon charge asymmetry in inclusive $pp \to W + X$ production at $\sqrt{s}$=7 TeV and an improved determination of light parton distribution functions*, Phys. Rev. D **90** (2014) 032004, `arXiv:1312.6283`.
